# Supplementary material for: Tachikuma: Understading Complex Interactions with Multi-Character and Novel Objects by Large Language Models
Source: arXiv:2307.12573 source file (2023-07-24)
Supplement: Supplementary file 1 [file supp.tex]

`Based on the above TRPG game record, which characters or NPC existed in current scenarios. Which character or NPC will carry out activities next? The team does not need to be listed separately. Strictly follow the format of "<Character name1>, <Character name2>, <Character name3>, ......" with different character names separated by a space. Remember to avoid to outputting 'None', 'Non', or any other similar non-action contents. Do not output DM and DM's actions. Do not output contents without any actions. Do not output any other content, do not output excess serial numbers and annotations. Each character appears and acts once at most. No need to explain the reason.'

What kind of skills are needed for the mentioned characters to carry out corresponding activities? What kind of attribute or other judgment does this skill need? Strictly follow the format of "<Character name>: <Skill>, <Attribute or other judgment>\\n" to output all possible characters and actions, such as "Morgan: Perception, Wisdom\\nArchie: Attack, Attack", with a line break between different characters. Do not output contents, if the character would not carry out activities or actions. Remember to avoid to outputting 'None', 'Non', or any other similar non-action contents. Do not output any other content, do not output excess serial numbers and annotations. Both the skill and attribute are predefined as a single word. Skills are one of the following: Strength, Athletics, Dexterity, Acrobatics, Sleight of Hand, Stealth, Constitution, Intelligence, Arcana, History, Investigation, Detect, Nature, Religion, Wisdom, Animal Handling, Insight, Medicine, Perception, Survival, Charisma, Deception, Intimidation, Performance, and Persuasion. Attribute or other judgments are one of the following: Strength, Dexterity, Constitution, Intelligence, Wisdom, Charisma, Initiative, Attack, Defense. Each character can appear and act at most once. There is no need to explain the reason.'

\begin{table}[]
	\begin{center}
	\resizebox{0.98\columnwidth}{!}
            {
                \begin{tabular}{|l|llll|llll|}
                \hline
                \multicolumn{1}{|c|}{\multirow{2}{*}{Prompting Method}} & \multicolumn{4}{c|}{Chinese Version}                                                                    & \multicolumn{4}{c|}{English Version}                                                                    \\ \cline{2-9} 
                \multicolumn{1}{|c|}{}                                  & \multicolumn{1}{c|}{CP} & \multicolumn{1}{c|}{CR} & \multicolumn{1}{c|}{CSP} & \multicolumn{1}{c|}{CSR} & \multicolumn{1}{c|}{CP} & \multicolumn{1}{c|}{CR} & \multicolumn{1}{c|}{CSP} & \multicolumn{1}{c|}{CSR} \\ \hline \hline 
                template prompt                                         & \multicolumn{1}{l|}{}   & \multicolumn{1}{l|}{26.81}   & \multicolumn{1}{l|}{}    &    9.20                      & \multicolumn{1}{l|}{}   & \multicolumn{1}{l|}{}   & \multicolumn{1}{l|}{}    &                          \\ \hline
                template prompt + zcot                                  & \multicolumn{1}{l|}{}   & \multicolumn{1}{l|}{}   & \multicolumn{1}{l|}{}    &                          & \multicolumn{1}{l|}{}   & \multicolumn{1}{l|}{}   & \multicolumn{1}{l|}{}    &                          \\ \hline
                char prompt + char prompt                               & \multicolumn{1}{l|}{}   & \multicolumn{1}{l|}{45.76}   & \multicolumn{1}{l|}{}    &    23.13                      & \multicolumn{1}{l|}{}   & \multicolumn{1}{l|}{}   & \multicolumn{1}{l|}{}    &                          \\ \hline
                pre-char prompt + char prompt + sta predictor           & \multicolumn{1}{l|}{}   & \multicolumn{1}{l|}{}   & \multicolumn{1}{l|}{}    &                          & \multicolumn{1}{l|}{}   & \multicolumn{1}{l|}{}   & \multicolumn{1}{l|}{}    &                          \\ \hline
                pre-char prompt + char prompt + sc prompt               & \multicolumn{1}{l|}{}   & \multicolumn{1}{l|}{}   & \multicolumn{1}{l|}{}    &                          & \multicolumn{1}{l|}{}   & \multicolumn{1}{l|}{}   & \multicolumn{1}{l|}{}    &                          \\ \hline
                pre-char prompt + char prompt + sc prompt + zcot        & \multicolumn{1}{l|}{}   & \multicolumn{1}{l|}{}   & \multicolumn{1}{l|}{}    &                          & \multicolumn{1}{l|}{}   & \multicolumn{1}{l|}{}   & \multicolumn{1}{l|}{}    &                          \\ \hline
                \end{tabular}
            }
        \end{center}
        \caption{GPT-3.5 Evaluation}
\end{table}

\begin{table}[]
	\begin{center}
	\resizebox{0.98\columnwidth}{!}
            {
                \begin{tabular}{|l|llll|llll|}
                \hline
                \multicolumn{1}{|c|}{\multirow{2}{*}{Prompting Method}} & \multicolumn{4}{c|}{Chinese Version}                                                                    & \multicolumn{4}{c|}{English Version}                                                                    \\ \cline{2-9} 
                \multicolumn{1}{|c|}{}                                  & \multicolumn{1}{c|}{CP} & \multicolumn{1}{c|}{CR} & \multicolumn{1}{c|}{CSP} & \multicolumn{1}{c|}{CSR} & \multicolumn{1}{c|}{CP} & \multicolumn{1}{c|}{CR} & \multicolumn{1}{c|}{CSP} & \multicolumn{1}{c|}{CSR} \\ \hline \hline 
                template prompt                                         & \multicolumn{1}{l|}{}   & \multicolumn{1}{l|}{26.81}   & \multicolumn{1}{l|}{}    &    9.20                      & \multicolumn{1}{l|}{}   & \multicolumn{1}{l|}{}   & \multicolumn{1}{l|}{}    &                          \\ \hline
                template prompt + zcot                                  & \multicolumn{1}{l|}{}   & \multicolumn{1}{l|}{}   & \multicolumn{1}{l|}{}    &                          & \multicolumn{1}{l|}{}   & \multicolumn{1}{l|}{}   & \multicolumn{1}{l|}{}    &                          \\ \hline
                char prompt + char prompt                               & \multicolumn{1}{l|}{}   & \multicolumn{1}{l|}{45.76}   & \multicolumn{1}{l|}{}    &    23.13                      & \multicolumn{1}{l|}{}   & \multicolumn{1}{l|}{}   & \multicolumn{1}{l|}{}    &                          \\ \hline
                pre-char prompt + char prompt + sta predictor           & \multicolumn{1}{l|}{}   & \multicolumn{1}{l|}{}   & \multicolumn{1}{l|}{}    &                          & \multicolumn{1}{l|}{}   & \multicolumn{1}{l|}{}   & \multicolumn{1}{l|}{}    &                          \\ \hline
                pre-char prompt + char prompt + sc prompt               & \multicolumn{1}{l|}{}   & \multicolumn{1}{l|}{}   & \multicolumn{1}{l|}{}    &                          & \multicolumn{1}{l|}{}   & \multicolumn{1}{l|}{}   & \multicolumn{1}{l|}{}    &                          \\ \hline
                pre-char prompt + char prompt + sc prompt + zcot        & \multicolumn{1}{l|}{}   & \multicolumn{1}{l|}{}   & \multicolumn{1}{l|}{}    &                          & \multicolumn{1}{l|}{}   & \multicolumn{1}{l|}{}   & \multicolumn{1}{l|}{}    &                          \\ \hline
                \end{tabular}
            }
        \end{center}
        \caption{GPT-4 Evaluation}
\end{table}

\begin{table}[]
	\begin{center}
	\resizebox{0.98\columnwidth}{!}
            {
                \begin{tabular}{|l|llll|llll|}
                \hline
                \multicolumn{1}{|c|}{\multirow{2}{*}{Prompting Method}} & \multicolumn{4}{c|}{Chinese Version}                                                                    & \multicolumn{4}{c|}{English Version}                                                                    \\ \cline{2-9} 
                \multicolumn{1}{|c|}{}                                  & \multicolumn{1}{c|}{CP} & \multicolumn{1}{c|}{CR} & \multicolumn{1}{c|}{CSP} & \multicolumn{1}{c|}{CSR} & \multicolumn{1}{c|}{CP} & \multicolumn{1}{c|}{CR} & \multicolumn{1}{c|}{CSP} & \multicolumn{1}{c|}{CSR} \\ \hline \hline 
                template prompt                                         & \multicolumn{1}{l|}{}   & \multicolumn{1}{l|}{26.81}   & \multicolumn{1}{l|}{}    &    9.20                      & \multicolumn{1}{l|}{}   & \multicolumn{1}{l|}{}   & \multicolumn{1}{l|}{}    &                          \\ \hline
                template prompt + zcot                                  & \multicolumn{1}{l|}{}   & \multicolumn{1}{l|}{}   & \multicolumn{1}{l|}{}    &                          & \multicolumn{1}{l|}{}   & \multicolumn{1}{l|}{}   & \multicolumn{1}{l|}{}    &                          \\ \hline
                char prompt + char prompt                               & \multicolumn{1}{l|}{}   & \multicolumn{1}{l|}{45.76}   & \multicolumn{1}{l|}{}    &    23.13                      & \multicolumn{1}{l|}{}   & \multicolumn{1}{l|}{}   & \multicolumn{1}{l|}{}    &                          \\ \hline
                pre-char prompt + char prompt + sta predictor           & \multicolumn{1}{l|}{}   & \multicolumn{1}{l|}{}   & \multicolumn{1}{l|}{}    &                          & \multicolumn{1}{l|}{}   & \multicolumn{1}{l|}{}   & \multicolumn{1}{l|}{}    &                          \\ \hline
                pre-char prompt + char prompt + sc prompt               & \multicolumn{1}{l|}{}   & \multicolumn{1}{l|}{}   & \multicolumn{1}{l|}{}    &                          & \multicolumn{1}{l|}{}   & \multicolumn{1}{l|}{}   & \multicolumn{1}{l|}{}    &                          \\ \hline
                pre-char prompt + char prompt + sc prompt + zcot        & \multicolumn{1}{l|}{}   & \multicolumn{1}{l|}{}   & \multicolumn{1}{l|}{}    &                          & \multicolumn{1}{l|}{}   & \multicolumn{1}{l|}{}   & \multicolumn{1}{l|}{}    &                          \\ \hline
                \end{tabular}
            }
        \end{center}
        \caption{ChatGLM Evaluation}
\end{table}

\begin{table}[]
	\begin{center}
	\resizebox{0.98\columnwidth}{!}
            {
                \begin{tabular}{|l|llll|llll|}
                \hline
                \multicolumn{1}{|c|}{\multirow{2}{*}{Prompting Method}} & \multicolumn{4}{c|}{Chinese Version}                                                                    & \multicolumn{4}{c|}{English Version}                                                                    \\ \cline{2-9} 
                \multicolumn{1}{|c|}{}                                  & \multicolumn{1}{c|}{CP} & \multicolumn{1}{c|}{CR} & \multicolumn{1}{c|}{CSP} & \multicolumn{1}{c|}{CSR} & \multicolumn{1}{c|}{CP} & \multicolumn{1}{c|}{CR} & \multicolumn{1}{c|}{CSP} & \multicolumn{1}{c|}{CSR} \\ \hline \hline 
                template prompt                                         & \multicolumn{1}{l|}{}   & \multicolumn{1}{l|}{26.81}   & \multicolumn{1}{l|}{}    &    9.20                      & \multicolumn{1}{l|}{}   & \multicolumn{1}{l|}{}   & \multicolumn{1}{l|}{}    &                          \\ \hline
                template prompt + zcot                                  & \multicolumn{1}{l|}{}   & \multicolumn{1}{l|}{}   & \multicolumn{1}{l|}{}    &                          & \multicolumn{1}{l|}{}   & \multicolumn{1}{l|}{}   & \multicolumn{1}{l|}{}    &                          \\ \hline
                char prompt + char prompt                               & \multicolumn{1}{l|}{}   & \multicolumn{1}{l|}{45.76}   & \multicolumn{1}{l|}{}    &    23.13                      & \multicolumn{1}{l|}{}   & \multicolumn{1}{l|}{}   & \multicolumn{1}{l|}{}    &                          \\ \hline
                pre-char prompt + char prompt + sta predictor           & \multicolumn{1}{l|}{}   & \multicolumn{1}{l|}{}   & \multicolumn{1}{l|}{}    &                          & \multicolumn{1}{l|}{}   & \multicolumn{1}{l|}{}   & \multicolumn{1}{l|}{}    &                          \\ \hline
                pre-char prompt + char prompt + sc prompt               & \multicolumn{1}{l|}{}   & \multicolumn{1}{l|}{}   & \multicolumn{1}{l|}{}    &                          & \multicolumn{1}{l|}{}   & \multicolumn{1}{l|}{}   & \multicolumn{1}{l|}{}    &                          \\ \hline
                pre-char prompt + char prompt + sc prompt + zcot        & \multicolumn{1}{l|}{}   & \multicolumn{1}{l|}{}   & \multicolumn{1}{l|}{}    &                          & \multicolumn{1}{l|}{}   & \multicolumn{1}{l|}{}   & \multicolumn{1}{l|}{}    &                          \\ \hline
                \end{tabular}
            }
        \end{center}
        \caption{LLaMA Evaluation}
\end{table}
